# Supplementary material for: A Tilted Bowl Is Not a Slippery Slope: Compressing Looped Models
Source: arXiv:2609.39277 source file (2026-09-30)
Supplement: Supplementary file 1 [file appendix.tex]

% ============================================================
% Appendix
% TRM Quantization Paper — EMNLP 2026 Industry Track
% ============================================================

\appendix

\begin{redpar}
\noindent\textbf{Legacy appendix from the Sep 13 EMNLP draft, unrevised.} Kept for its tables and job-id provenance. Known
problems: device INT8/INT4 rows time $H{=}3$ step graphs whose activations are 8-bit (host simulation: Sudoku-MLP w8a8 solves
0/100); TFLM outputs are invalid (REDUCE\_SUM bug) and attention FVP cycle counts are invalid; HRM tables may mix $H$ (REWRITE\_NOTES
27); ``QAT cannot repair it'' is withdrawn (X5: naive QAT 0.0$\to$52.3); the energy appendix has no measurement; \textbf{every INT4 device latency and memory row is unverified}: INT4-weight graphs on the Hexagon
HTP compute the wrong function (disabled \texttt{QNN\_CastInt4ToInt8} op; REWRITE\_NOTES 49) and the Sep 10 INT4 rows were never correctness-checked. The results bank
(Part~\ref{part:results}) supersedes every overlapping number.
\end{redpar}

\section{Peak SRAM Memory Footprints}
\label{app:sram_footprint}

\begin{table}[h]
\centering
\small
\setlength{\tabcolsep}{4pt}
\begin{tabular}{@{}llll@{}}
\toprule
Figure & What it measures & Measured? & Reported in \\
\midrule
6.7\,MB    & INT8 backbone weights            & analytical & Table~\ref{tab:full_results} \\
6.51\,MB   & INT8 $+$ flash, weights only     & analytical & Table~\ref{tab:deployment} \\
3.26\,MB   & INT4 cal.\ $+$ flash, weights only & analytical & Table~\ref{tab:deployment} \\
4.7 / 4.5 / 3.2\,MB & 4-bit-weight graph flatbuffer (Maze/ARC backbone, Sudoku-attn, Sudoku-MLP) & measured & Appendix~\ref{app:mcu} \\
7.7 / 8.8 / 6.4\,MB & INT8 graph flatbuffer, same three & measured & Appendix~\ref{app:mcu} \\
9.51\,MB   & streaming peak, incl.\ activations & analytical & Table~\ref{tab:sram_footprints} \\
3.2--10.5\,MB & INT4 step, inference memory increase, three devices & measured & Table~\ref{tab:on_device_benchmarks} \\
1.3\,MB + 6.4\,MB flash & Sudoku-MLP INT8 step, Ethos-U55 SRAM (Vela) & measured & Appendix~\ref{app:mcu} \\
8.1\,MB    & Sudoku-MLP INT8 step, TFLite Micro arena (Cortex-M kernels) & measured & Appendix~\ref{app:mcu} \\
14--53\,MB & attention INT8 steps, TFLite Micro arena & measured & Appendix~\ref{app:mcu} \\
6\,MB      & INT4 step, process peak, QCS6490 NPU & measured & Table~\ref{tab:on_device_benchmarks} \\
97--112\,MB & phone process peak (runtime baseline 90--101\,MB) & measured   & Table~\ref{tab:on_device_benchmarks} \\
\bottomrule
\end{tabular}
\caption{Every memory figure this paper reports, what it covers, and whether it
was measured or derived. The weights-only rows exclude activations and carry
state. Of the measured rows, the inference increase is the step's own cost
(activations and scratch); the process peaks include the runtime, which is
4.5\,MB on the QCS6490 and 90--101\,MB on the Android phones
(\S\ref{app:latency}).}
\label{tab:memfigures}
\end{table}

For on-device edge deployment, we evaluate the peak memory footprint under two execution scenarios: a \emph{Full Load} scenario (where the entire backbone and intermediate activations/carries are stored in SRAM) and a \emph{Streaming} scenario (where only the current recursive step is loaded, leveraging single-puzzle flash loading of embedding tables). 

Table~\ref{tab:sram_footprints} compiles these peak SRAM requirements against a theoretical 8\,MB SRAM hardware budget limit.

\begin{table}[h]
\centering
\small
\begin{tabular}{lrrc}
\toprule
\textbf{Model / Variant} & \textbf{Streaming} & \textbf{Full Load} & \textbf{Fits 8\,MB? (Streaming)} \\
\midrule
ARC (FP32, no embed) & 27.31\,MB & 40.31\,MB & \ding{55} \\
ARC (INT8, no embed) & 9.51\,MB & 12.76\,MB & \ding{55} \\
Maze (FP32) & 27.31\,MB & 40.31\,MB & \ding{55} \\
Maze (INT8) & 9.51\,MB & 12.76\,MB & \ding{55} \\
Sudoku (FP32) & 11.08\,MB & 20.65\,MB & \ding{55} \\
Sudoku (INT8) & 3.06\,MB & 5.45\,MB & \ding{51} \\
\bottomrule
\end{tabular}
\caption{Peak memory footprint (SRAM) for deployable ONNX models, including
intermediate activations and carry state. Embedding layers are excluded
(no-embed) as they are streamed via flash loading. The 8\,MB target assumes
streaming mode. These activation-inclusive peaks complement the weights-only
analytical figures of Table~\ref{tab:deployment}.}
\label{tab:sram_footprints}
\end{table}

Under streaming execution, only the Sudoku (INT8) model fits within the
8\,MB SRAM budget (3.06\,MB streaming peak); the ARC and Maze INT8 models
peak at 9.51\,MB, so their 8\,MB fit is not yet demonstrated
(\S\ref{sec:deployment}).

\section{On-Device Hardware Benchmarks}
\label{app:latency}

Rather than relying purely on first-order analytical projections, we compile
one recursive inner step of the ARC-AGI-1 model (sequence length 900, the
official public checkpoint, puzzle embedding passed in as a graph input so
the table can be streamed from flash) and profile it on three physical edge
devices through Qualcomm AI Hub:
\begin{itemize}[leftmargin=*]
    \item \textbf{Samsung Galaxy S24}: Qualcomm Snapdragon 8 Gen 3 (SM8650, Hexagon v75 NPU).
    \item \textbf{Samsung Galaxy S22 5G}: Qualcomm Snapdragon 8 Gen 1 (SM8450, Hexagon v70 NPU).
    \item \textbf{Dragonwing RB3 Gen 2}: Qualcomm QCS6490 (Hexagon NPU, fixed-point only).
\end{itemize}

Every row in Table~\ref{tab:on_device_benchmarks} is one AI Hub profile job
whose identifier is given, so the compile report, the per-layer placement
and the runtime trace can be retrieved. All three precisions are compiled to
the same target, a QNN context binary, so the precision ladder is measured
on one runtime rather than across runtimes; the quantized rows also
quantize the graph inputs and outputs, which is what a fixed-point
deployment would ship. The controlled quantity is the per-\emph{step}
latency, which is depth-independent by construction; the per-puzzle latency
at the deployment depth of Table~\ref{tab:deployment} ($H{=}1$,
$n_\text{sup}{=}8$) is eight steps, e.g.\ 0.47\,s for INT4 on the S24.

Three things the table settles. First, \textbf{INT4 executes as INT4 and is
the fastest precision on every device that runs it}: 2.6$\times$ FP32 and
1.3$\times$ INT8 on the S24, 2.3$\times$ and 1.4$\times$ on the S22. An
earlier attempt to profile INT4 through the TF-Lite target reproduced FP32
latency exactly, because TF-Lite has no INT4 tensor type and the compiler
folds the quantize--dequantize pairs back to float; the QNN target has no
such fallback. Second, \textbf{the step's own memory is small on every device}. The
profile report separates the process peak while loading the model from the
increase during inference, and the two tell different stories. On the phones
the load peak is 90--101\,MB at every precision, including the INT4 graph:
that is the Android QNN runtime and its libraries, not the model, and
quantizing the graph I/O moves it by only 5--8\,MB. The increase during
inference, which is what the step's activations and scratch cost, is
8.5\,MB for INT4 on the S24 and 10.5\,MB on the S22, against 10.9 and
14.0\,MB for FP32; the analytical INT8 streaming peak of
Table~\ref{tab:sram_footprints} is 9.5\,MB. On the QCS6490, whose runtime
carries a 4.5\,MB load baseline, \textbf{the INT4 step runs in 6\,MB of peak
process memory}, 3.2\,MB of it inference; that device accepts no
floating-point tensor anywhere in the graph, so FP32 falls back to its GPU
(1{,}341\,ms, 673\,MB, reported for completeness) and INT8 does not compile
because AI Hub's INT8 recipe leaves the recursion's residual add in FP16.
Third, \textbf{the phones' 97--112\,MB process peak is therefore a runtime
figure}, reported as measured and not read as an SRAM footprint; the
model-attributable figure on those devices is the inference increase.

\begin{table*}[t]
\centering
\small
\begin{tabular}{llrrrrl}
\toprule
\textbf{Device} & \textbf{Precision} & \textbf{Step (ms)} & \textbf{Load (MB)} & \textbf{Infer.\ $+$ (MB)} & \textbf{Peak (MB)} & \textbf{Unit} \\
\midrule
Galaxy S24 & FP32$^{\ddagger}$ & 151.29 & 101 & 10.9 & 112 & NPU \\
Galaxy S24 & INT8 & 75.11 & 97 & 8.4 & 104 & NPU \\
Galaxy S24 & INT4 & \textbf{58.29} & 97 & \textbf{8.5} & 104 & NPU \\
\midrule
Galaxy S22 & FP32$^{\ddagger}$ & 319.81 & 91 & 14.0 & 103 & NPU \\
Galaxy S22 & INT8 & 184.90 & 90 & 11.0 & 97 & NPU \\
Galaxy S22 & INT4 & \textbf{136.64} & 90 & \textbf{10.5} & 97 & NPU \\
\midrule
Dragonwing RB3 & FP32 & 1341.21 & 1146 & 429 & 673 & GPU$^{\S}$ \\
Dragonwing RB3 & INT8 & \multicolumn{5}{l}{does not compile fixed-point (FP16 residual add)} \\
Dragonwing RB3 & INT4 & \textbf{290.87} & 4.5 & \textbf{3.2} & \textbf{6} & NPU \\
\bottomrule
\end{tabular}
\caption{The phones' 100\,MB is the runtime, not the model: the step's own
memory (\emph{Infer.\ $+$}) is 3--14\,MB on every device. One ARC-AGI-1
inner step (sequence length 900, every layer on the named unit) profiled on
physical devices through Qualcomm AI Hub. \emph{Load} is the process peak
while loading runtime and model, \emph{Infer.\ $+$} the largest increase
during inference (activations and scratch), \emph{Peak} the process peak
during inference. Phone rows are QNN context binaries with quantized I/O
for INT8 and INT4 (float-I/O variants run within 1\,ms). $^{\ddagger}$FP32
executes as FP16 on the Hexagon vector engine, the phones' float path.
$^{\S}$The QCS6490 NPU is fixed-point only, so FP32 runs on its GPU. The
profile job identifiers behind every row are listed in
Appendix~\ref{app:jobids} for retrieval.}
\label{tab:on_device_benchmarks}
\end{table*}

\subsection{Provenance of the on-device rows}
\label{app:jobids}

Every row of Table~\ref{tab:on_device_benchmarks} is one Qualcomm AI Hub
profile job, from which the compile report, per-layer unit placement and
runtime trace can be retrieved at
\texttt{aihub.qualcomm.com/jobs/<id>}. In table order: S24 FP32
\texttt{jgd3ljl6p}, INT8 \texttt{jprl3e87p}, INT4 \texttt{j5m0x3q9g}; S22
FP32 \texttt{jpx42w28g}, INT8 \texttt{jp2ryl0qg}, INT4 \texttt{jgnzv3lqg};
RB3 FP32 \texttt{jp8xvnlog}, INT8 compile \texttt{jg9meekv5} (failed), INT4
\texttt{jp8xvvlkg}. The float-I/O phone profiles are \texttt{jglxrdnmg},
\texttt{jgk4m1jnp} (S24 INT8, INT4) and \texttt{j567lx6yp},
\texttt{j5qyonjog} (S22). The per-task rows of
Table~\ref{tab:seqlen_ondevice}, S24 then S22, FP32 then INT8 then INT4,
and last the QCS6490 INT4 profile: Maze-Hard \texttt{jgzldxoo5},
\texttt{jg9zn3jwp}, \texttt{jgdd1rz6g}, \texttt{j5wl6d23p},
\texttt{jp1nzdy8g}, \texttt{jpxlo7d8p}, \texttt{jgk2xl8vg}; Sudoku
TRM-attn \texttt{jp8ey7lxp}, \texttt{jp0m012ng}, \texttt{jp0m01d0g},
\texttt{jgk2xyj2g}, \texttt{jp8ey3mop}, \texttt{jp2ry746g},
\texttt{jpyo34q05}; Sudoku TRM-MLP \texttt{jgk2xlyng}, \texttt{jglym00m5},
\texttt{j5qlq7vep}, \texttt{j5qlq72op}, \texttt{j568433yg},
\texttt{j56843wng}, \texttt{jgjrn0q1p}.

\subsection{MCU-tier compilation: Vela and TensorFlow Lite Micro}
\label{app:mcu}

Each inner step (one full recursion of the inner model, the unit the
phones profile) was exported to TFLite in FP32 with litert-torch and
quantized post-training on the finished graph with the AI Edge Quantizer
(static INT8: per-channel weights, 8-bit activations, eight unit-scale
random calibration inputs), then (a) compiled with Vela 5.2 for the
Ethos-U55-256 under the \texttt{Ethos\_U55\_High\_End\_Embedded} system
configuration (500\,MHz) in shared-SRAM mode, the Corstone-300 layout, which
reports the SRAM and flash the compiled graph occupies and a cycle estimate
that Arm documents as cycle-approximate for the NPU, and (b) loaded by
TensorFlow Lite Micro's recording allocator, which reports the tensor arena
the same graph needs on a Cortex-M's own reference kernels (head:
activations; tail: persistent per-operator buffers). Every weight tensor in
the audited graphs is INT8; the flash column is the flatbuffer size.

\begin{center}
\small
\setlength{\tabcolsep}{4pt}
\begin{tabular}{@{}lrrrrrrr@{}}
\toprule
 & & \multicolumn{4}{c}{Ethos-U55-256 (Vela)} & \multicolumn{2}{c}{Cortex-M55 kernels} \\
\cmidrule(lr){3-6}\cmidrule(lr){7-8}
INT8 step & flash & SRAM & ops on NPU & GMAC & step & TFLM arena & head / tail \\
\midrule
Sudoku, TRM-MLP ($T{=}81$)   & 6.4\,MB & \textbf{1.3\,MB} & 99.8\% & 12.8 & \textbf{312\,ms} & 8.1\,MB & 6.3 / 1.8 \\
Sudoku, TRM-attn ($T{=}81$)  & 8.8\,MB & 0.9\,MB & 99.9\% & 14.3 & 975\,ms & 14.1\,MB & 7.7 / 6.4 \\
Maze, TRM-attn ($T{=}900$)   & 7.7\,MB$^{\ast}$ & 55\,MB & 99.9\% & 120.0 & 35.4\,s & 53\,MB & 23 / 30 \\
\bottomrule
\end{tabular}
\end{center}

With a fully integer graph Vela places all but two operators of every step
on the NPU, so its cycle estimate covers the whole step. The MLP-mixing
Sudoku step is flash-bandwidth bound (93\,MB of weights streamed per step
at 0.47\,GB/s account for 98 of its 156\,M cycles) and reaches 32\% of the
array's 128\,GMAC/s; the attention step at the same length costs
3.1$\times$ the cycles for 1.1$\times$ the MACs, because the $97\times97$
per-head attention products run the 256-MAC array at low utilisation, and
its persistent arena tail is the reference kernels' attention scratch. At
$T{=}900$ the attention maps ($8\times916\times916$ per layer) exceed the
SRAM in either runtime; $^{\ast}$Vela spills them to off-chip memory (776\,MB
in this configuration, which has no DRAM) and the step runs at 2.6\% of the
array. The CPU-only analytical bound for the Sudoku MLP step, 12.8\,GMAC at
a Cortex-M55's roughly 1\,GMAC/s, is about 13\,s, 40$\times$ the NPU
estimate; we report it only as that bound. The same pipeline with 4-bit
per-channel weights (the calibrated-INT4 configuration) gives flatbuffers
of 3.2\,MB (Sudoku-MLP), 4.5\,MB (Sudoku-attn) and 4.7\,MB (Maze); neither
Vela nor the reference kernels execute 4-bit weights, so those are flash
footprints only. The graphs are calibrated on unit-scale random inputs and
are memory and compute artefacts, not accuracy artefacts; static-INT8
accuracy is measured in the harness (Appendix~\ref{app:static_dynamic}).

\paragraph{Execution on the Corstone-300 virtual platform.} To check the
Vela estimate against an execution, we ran the Vela-compiled Sudoku-MLP
step on Arm's Corstone-300 Fixed Virtual Platform (Cortex-M55 with
Ethos-U55-256) through the ML embedded evaluation kit's inference runner
(GNU 13.2; the kit's op resolver extended with the embedding lookup, token
inputs held in vocabulary). The application allocates a 1{,}300{,}644-byte
arena on the target, matching Vela's 1.27\,MB, and the NPU performance
counters report 166.26\,M cycles for one step (166.26\,M active, 809 idle),
332\,ms at 500\,MHz, 7\% above Vela's static 155.83\,M-cycle estimate. Arm
documents the Ethos-U model of this platform as cycle-approximate and its
Cortex-M model as not cycle-accurate, so the NPU cycle count is the
quantity we report, and it covers the 99.8\% of operators that run on the
NPU. The same application built without the NPU allocates an
8{,}022{,}660-byte arena on the target for the 1{,}377-operator
reference-kernel graph and runs it to completion in 11.5\,G Cortex-M55
instructions, a check of the TensorFlow Lite Micro figure and of the graph
rather than a timing, since the platform does not model Cortex-M cycles.

\subsection{Sequence-Length Dependent Quantization Penalty}
\label{app:seq_len_penalty}

The phone rows of Table~\ref{tab:on_device_benchmarks} are QNN context
binaries executed on the Hexagon processor with every layer placed on the
NPU. Graphs labeled ``FP32'' execute in FP16 on the Hexagon vector engine
(HVX), which is the phones' floating-point path; INT8 and INT4 graphs execute
on the HTP tensor units with quantize--dequantize (QDQ) boundaries at node
interfaces. The QCS6490's HTP is fixed-point only, so the RB3 FP32 row runs
on that device's GPU through the TF-Lite delegate and is not comparable to
its INT4 row.

Whether INT8 pays on the NPU depends on the sequence length, and we measured
both regimes. Table~\ref{tab:seqlen_ondevice} profiles the inner step of
each task on the two phones with the same pipeline as
Table~\ref{tab:on_device_benchmarks}. At $T{=}900$ (ARC-AGI-1 and Maze-Hard
share the backbone and the length; the exported graph carries 16 further
puzzle-embedding positions) the projection matrices are large,
$900\times512$ by $512\times2048$, the step is compute-bound, and moving it
from the HVX FP16 pipeline to the INT8 tensor units pays 2.1$\times$ on the
S24 and 1.8$\times$ on the S22. At Sudoku length ($T{=}81$, 97 positions
exported) a step is about 25\,MFLOPs, the matrix products are too small to
fill the INT8 execution blocks, and the fixed dispatch and QDQ cost per node
dominates: \textbf{INT8 attention is 26\% slower than FP16 on the S24} and
8\% slower on the S22. The MLP-mixing step, whose token-mixing layers
(388\,KB/194\,KB) are also below the tensor unit's tile size, is within 10\%
of FP16 on the S24 and gains only on the older S22 (1.7$\times$). INT4 still
pays at the short length, 1.1--2.2$\times$, because it halves the weight
fetch again while the per-node cost stays where it was, and it pays
2.5--2.7$\times$ at $T{=}900$. On the QCS6490 the INT4 step runs in a
7.2\,MB process for Maze and a 4.6\,MB process for either Sudoku mixer.
Per-step memory on the phones does not depend on the mixer or the task: the
inference increase is 7--12\,MB for every graph on top of the 86--95\,MB
runtime, with one exception we report as measured, the Maze INT4 profile on
the S24 (20\,MB; the same binary on the S22 reports 9.8\,MB).

\begin{table}[h]
\centering
\small
\setlength{\tabcolsep}{3.5pt}
\begin{tabular}{@{}lrrrrrrrrr@{}}
\toprule
 & & \multicolumn{3}{c}{Galaxy S24 (ms)} & \multicolumn{3}{c}{Galaxy S22 (ms)} & \multicolumn{2}{c}{QCS6490 INT4} \\
\cmidrule(lr){3-5}\cmidrule(lr){6-8}\cmidrule(lr){9-10}
Step & $T$ & FP32 & INT8 & INT4 & FP32 & INT8 & INT4 & ms & peak MB \\
\midrule
ARC-AGI-1, TRM-attn  & 900 & 151.3 & 75.1 (2.0$\times$) & 58.3 (2.6$\times$) & 319.8 & 184.9 (1.7$\times$) & 136.6 (2.3$\times$) & 290.9 & 6.0 \\
Maze-Hard, TRM-attn  & 900 & 150.1 & 71.8 (2.1$\times$) & 56.3 (2.7$\times$) & 319.6 & 182.6 (1.8$\times$) & 127.2 (2.5$\times$) & 275.9 & 7.2 \\
Sudoku, TRM-attn     & 81  & 9.06  & \textbf{11.39 (0.8$\times$)} & 7.14 (1.3$\times$) & 22.67 & 24.50 (0.9$\times$) & 20.24 (1.1$\times$) & 60.0 & 4.6 \\
Sudoku, TRM-MLP      & 81  & 11.32 & 10.26 (1.1$\times$) & 6.77 (1.7$\times$) & 38.16 & 22.64 (1.7$\times$) & 17.46 (2.2$\times$) & 49.4 & 4.6 \\
\bottomrule
\end{tabular}
\caption{INT8 pays only at $T{=}900$; INT4 pays at both lengths. One inner
step per task on the NPU through Qualcomm AI Hub, FP32 executing as FP16
on the Hexagon vector engine, INT8 and INT4 as quantized-I/O context
binaries; the ratio is FP32 over quantized latency. The QCS6490 columns
give the INT4 step and its process peak during inference. ARC rows repeat
Table~\ref{tab:on_device_benchmarks}; job identifiers in
Appendix~\ref{app:jobids}.}
\label{tab:seqlen_ondevice}
\end{table}



\subsection{Static vs.\ Dynamic Quantization}
\label{app:static_dynamic}

Dynamic quantization preserves full-precision accuracy on every task. Static
quantization does not, and Sudoku-Extreme recovers only under selective
operator exclusion: leaving activation and carry-state updates in FP32 and
quantizing only the \texttt{MatMul}/\texttt{Gemm} weights. The trade-off
matters for deployment: dynamic quantization is the robust out-of-the-box path
for recursive models, but NPU accelerators require static, pre-allocated tensor
boundaries, so the static path and its operator exclusions are what on-device
execution inherits (\S\ref{app:seq_len_penalty}). Where the static loss
comes from is measured on the official ARC checkpoint ($n_\text{sup}{=}16$,
$H{=}3$, bf16 forward, all 368{,}150 augmented test rows): FP32 gives
3.46\% token-exact rows and 73.84\% cell accuracy; per-channel INT8
weights alone give 3.46\% and 73.85\%; adding static INT8 activations
calibrated on 96 rows gives 2.72\% and 71.21\%. Weight quantization is
lossless at this precision and the activation quantizer is the whole
static gap. These are token-level figures over augmented rows, not the
per-task pass@1 of Table~\ref{tab:arc_official}, whose protocol scores
each task once.

\section{Full Precision × Task Results}
\label{app:full_results}

\begin{table*}[h]
\centering
\small
\begin{tabular}{lrrc}
\toprule
\textbf{Configuration} & \textbf{Weights} & \textbf{GFLOPs/puzzle} & \textbf{Fits 8\,MB (weights)?} \\
\midrule
FP32, $H{=}3$, $n{=}16$, full emb.                  & $\sim$126\,MB & 3{,}000   & \ding{55} \\
\textbf{INT8, $H{=}1$, $n{=}8$, flash loading}      & \textbf{6.51\,MB}  & \textbf{500}   & \ding{51} \\
\textbf{INT4 calibrated, $H{=}1$, $n{=}8$, flash}    & \textbf{3.26\,MB}  & \textbf{500}   & \ding{51} \\
\bottomrule
\end{tabular}
\caption{Only the INT8 and calibrated-INT4 backbones with flash-loaded
embeddings fit the 8\,MB weight budget on ARC-AGI-1, at one sixth of the
FP32 compute. Deployment configurations per puzzle; analytical,
weights-only; excludes activations and carry state (see
Table~\ref{tab:sram_footprints} for activation-inclusive streaming peaks).
Bold marks viable targets. Figures show backbone-only weight footprint (ARC
embedding handled via flash loading). On-device latencies are measured
directly on physical hardware (Table~\ref{tab:on_device_benchmarks}).
Per-channel calibrated INT4 recovers near-FP32 accuracy without retraining
(\S\ref{sec:recovery}). The exported 4-bit graph of this backbone measures
4.7\,MB of flash with embeddings and scales (Appendix~\ref{app:mcu}); the
INT4 step itself is measured on device at 58\,ms (S24) and 291\,ms in 6\,MB
of peak process memory (QCS6490 NPU), Table~\ref{tab:on_device_benchmarks}.}
\label{tab:deployment}
\end{table*}

Table~\ref{tab:full_results} reports full-system accuracy across all
precision levels and tasks at the evaluated recursive depth.

\begin{table*}[h]
\centering
\small
\begin{tabular}{llrrrrrr}
\toprule
 & & \multicolumn{2}{c}{\textbf{ARC-AGI-1}} & \multicolumn{2}{c}{\textbf{Maze-Hard}} & \multicolumn{2}{c}{\textbf{Sudoku-Extreme}} \\
\cmidrule(lr){3-4}\cmidrule(lr){5-6}\cmidrule(lr){7-8}
\textbf{Precision} & \textbf{SRAM} & \textit{PExact} & \textit{CellAcc} & \textit{PExact} & \textit{CellAcc} & \textit{PExact} & \textit{CellAcc} \\
\midrule
FP32$^\dagger$  & 26.7\,MB & 36.00\% & 88.22\% & 86.80\% & 99.52\% & 69.10\% & 87.47\% \\
FP16            & 13.3\,MB & 36.00\% & 87.57\% & 87.00\% & 99.53\% & 68.50\% & 87.20\% \\
INT8            & 6.7\,MB  & 36.00\% & 87.62\% & 87.00\% & 99.53\% & 69.10\% & 87.51\% \\
INT4 na\"ive    & 3.3\,MB  & 25.50\% & 84.80\% & 86.40\% & 99.50\% & 5.30\%  & 66.02\% \\
\bottomrule
\end{tabular}
\caption{INT8 is lossless on all three tasks and na\"ive INT4 is
task-dependent: ten points on ARC-AGI-1, nothing on Maze-Hard, collapse on
Sudoku-Extreme. Full-system precision × task accuracy at the evaluated
recursive depth, \emph{submission protocol} ($H{=}3$, $n_\text{sup}{=}10$,
bf16 forward, first-$N$ subsets); the corrected-protocol headline figures are
in Table~\ref{tab:corrected}, and the official-checkpoint ARC figures in
Table~\ref{tab:arc_official}. ARC-AGI-1 public evaluation set (400 tasks),
single-pass (no test-time augmentation). SRAM shows backbone-only footprint
(ARC embedding handled via flash loading). $^\dagger$FP32 rows executed a bf16
forward pass; SRAM at FP32 precision.}
\label{tab:full_results}
\end{table*}

\section{Detailed Recursive Sweep Grids}
\label{app:sweeps_detail}

We report the complete multi-variant validation sweeps across combinations of recursive steps ($n$) and precision modes on GPU (CUDA) for all three architectures. Tables~\ref{tab:arc_sweep_detail}, \ref{tab:maze_sweep_detail}, and \ref{tab:sudoku_sweep_detail} present these complete grids, including exact match accuracy and cell accuracy.

\begin{table*}[p]
\centering
\small
\begin{tabular}{lclrrrrr}
\toprule
\textbf{Precision} & \textbf{$H$} & \textbf{Metric} & \textbf{$n=1$} & \textbf{$n=2$} & \textbf{$n=4$} & \textbf{$n=8$} & \textbf{$n=16$} \\
\midrule
FP32 (bf16) & 3 & Exact & 0.2850 & 0.3600 & 0.3575 & 0.3575 & 0.3600 \\
            &   & Cell & 0.8762 & 0.8839 & 0.8764 & 0.8760 & 0.8757 \\
            & 1 & Exact & 0.0025 & 0.0750 & 0.3425 & 0.3575 & 0.3550 \\
            &   & Cell & 0.5410 & 0.7954 & 0.8825 & 0.8832 & 0.8762 \\
\midrule
FP16        & 3 & Exact & 0.2850 & 0.3600 & 0.3575 & 0.3600 & 0.3625 \\
            &   & Cell & 0.8762 & 0.8838 & 0.8765 & 0.8763 & 0.8755 \\
            & 1 & Exact & 0.0025 & 0.0750 & 0.3450 & 0.3550 & 0.3575 \\
            &   & Cell & 0.5410 & 0.7953 & 0.8825 & 0.8831 & 0.8773 \\
\midrule
INT8 (bnb)  & 3 & Exact & 0.2850 & 0.3575 & 0.3575 & 0.3600 & 0.3600 \\
            &   & Cell & 0.8760 & 0.8837 & 0.8827 & 0.8842 & 0.8670 \\
            & 1 & Exact & 0.0025 & 0.0750 & 0.3425 & 0.3525 & 0.3625 \\
            &   & Cell & 0.5415 & 0.7953 & 0.8827 & 0.8835 & 0.8767 \\
\midrule
INT4 (naive)& 3 & Exact & 0.1575 & 0.2700 & 0.2675 & 0.2625 & 0.2575 \\
            &   & Cell & 0.8372 & 0.8626 & 0.8473 & 0.8430 & 0.8322 \\
            & 1 & Exact & 0.0000 & 0.0225 & 0.2525 & 0.2650 & 0.2600 \\
            &   & Cell & 0.3954 & 0.7148 & 0.8582 & 0.8494 & 0.8415 \\
\bottomrule
\end{tabular}
\caption{On ARC-AGI-1, FP32, FP16 and INT8 are indistinguishable at every
depth (36\% exact from $n{=}2$ at $H{=}3$, from $n{=}4$ at $H{=}1$) and
na\"ive INT4 costs about ten points at every depth (26--27\%), so the
depth axis cannot buy back what the precision axis loses. Full recursive
sweep (seq\_len = 900) across $H$ (outer cycles), $n$ (supervision steps)
and precision.}
\label{tab:arc_sweep_detail}
\end{table*}

\begin{table*}[p]
\centering
\small
\begin{tabular}{lclrrrrr}
\toprule
\textbf{Precision} & \textbf{$H$} & \textbf{Metric} & \textbf{$n=1$} & \textbf{$n=2$} & \textbf{$n=4$} & \textbf{$n=8$} & \textbf{$n=16$} \\
\midrule
FP32 (bf16) & 3 & Exact & 0.7850 & 0.8670 & 0.8700 & 0.8700 & 0.8700 \\
            &   & Cell & 0.9940 & 0.9953 & 0.9953 & 0.9953 & 0.9953 \\
            & 1 & Exact & 0.0000 & 0.1390 & 0.8440 & 0.8690 & 0.8700 \\
            &   & Cell & 0.4363 & 0.9808 & 0.9949 & 0.9953 & 0.9953 \\
\midrule
FP16        & 3 & Exact & 0.7850 & 0.8670 & 0.8700 & 0.8700 & 0.8700 \\
            &   & Cell & 0.9940 & 0.9953 & 0.9953 & 0.9953 & 0.9953 \\
            & 1 & Exact & 0.0000 & 0.1380 & 0.8440 & 0.8700 & 0.8700 \\
            &   & Cell & 0.4362 & 0.9808 & 0.9949 & 0.9953 & 0.9953 \\
\midrule
INT8 (bnb)  & 3 & Exact & 0.7830 & 0.8680 & 0.8710 & 0.8700 & 0.8700 \\
            &   & Cell & 0.9940 & 0.9953 & 0.9953 & 0.9953 & 0.9953 \\
            & 1 & Exact & 0.0000 & 0.1380 & 0.8450 & 0.8690 & 0.8700 \\
            &   & Cell & 0.4333 & 0.9808 & 0.9949 & 0.9953 & 0.9953 \\
\midrule
INT4 (naive)& 3 & Exact & 0.7660 & 0.8610 & 0.8640 & 0.8640 & 0.8640 \\
            &   & Cell & 0.9934 & 0.9949 & 0.9950 & 0.9950 & 0.9950 \\
            & 1 & Exact & 0.0000 & 0.1580 & 0.8360 & 0.8630 & 0.8630 \\
            &   & Cell & 0.4734 & 0.9805 & 0.9945 & 0.9950 & 0.9950 \\
\bottomrule
\end{tabular}
\caption{Maze-Hard is indifferent to precision and saturates early: every
precision, na\"ive INT4 included, reaches 86--87\% exact by $n{=}2$ at
$H{=}3$ and by $n{=}8$ at $H{=}1$, so on this task depth can be traded for
precision freely. Full recursive sweep (seq\_len = 900) across $H$ (outer
cycles), $n$ (supervision steps) and precision.}
\label{tab:maze_sweep_detail}
\end{table*}

\begin{table*}[p]
\centering
\small
\begin{tabular}{lclrrrrr}
\toprule
\textbf{Precision} & \textbf{$H$} & \textbf{Metric} & \textbf{$n=1$} & \textbf{$n=2$} & \textbf{$n=4$} & \textbf{$n=8$} & \textbf{$n=16$} \\
\midrule
FP32 (bf16) & 3 & Exact & 0.2840 & 0.4960 & 0.6040 & 0.6690 & 0.7090 \\
            &   & Cell & 0.7640 & 0.8147 & 0.8474 & 0.8680 & 0.8810 \\
            & 1 & Exact & 0.0060 & 0.0210 & 0.3830 & 0.5470 & 0.6370 \\
            &   & Cell & 0.5527 & 0.6943 & 0.7856 & 0.8293 & 0.8563 \\
\midrule
FP16        & 3 & Exact & 0.2830 & 0.4960 & 0.6100 & 0.6700 & 0.7160 \\
            &   & Cell & 0.7639 & 0.8151 & 0.8488 & 0.8677 & 0.8851 \\
            & 1 & Exact & 0.0060 & 0.0210 & 0.3830 & 0.5480 & 0.6390 \\
            &   & Cell & 0.5526 & 0.6941 & 0.7856 & 0.8303 & 0.8574 \\
\midrule
INT8 (bnb)  & 3 & Exact & 0.2800 & 0.5010 & 0.6210 & 0.6790 & 0.7120 \\
            &   & Cell & 0.7643 & 0.8183 & 0.8524 & 0.8721 & 0.8816 \\
            & 1 & Exact & 0.0060 & 0.0210 & 0.3820 & 0.5540 & 0.6560 \\
            &   & Cell & 0.5528 & 0.6942 & 0.7852 & 0.8306 & 0.8638 \\
\midrule
INT4 (naive)& 3 & Exact & 0.0210 & 0.0290 & 0.0510 & 0.0550 & 0.0610 \\
            &   & Cell & 0.6277 & 0.6490 & 0.6524 & 0.6573 & 0.6597 \\
            & 1 & Exact & 0.0000 & 0.0120 & 0.0210 & 0.0370 & 0.0510 \\
            &   & Cell & 0.5612 & 0.6097 & 0.6375 & 0.6536 & 0.6555 \\
\bottomrule
\end{tabular}
\caption{Sudoku-Extreme keeps improving with depth and collapses under
na\"ive INT4: FP32, FP16 and INT8 track each other within a point at every
cell and rise from 28\% to 71\% exact as $n$ goes 1 to 16 at $H{=}3$, while
na\"ive INT4 never exceeds 6\% at any depth. Full recursive sweep
(seq\_len = 81) across $H$ (outer cycles), $n$ (supervision steps) and
precision.}
\label{tab:sudoku_sweep_detail}
\end{table*}

\section{Depth × Quantization Sweep (ARC-AGI-1)}
\label{app:depth_arc}

Table~\ref{tab:depth_arc} reports key ARC-AGI-1 depth configurations
(full-system, single-pass): INT8 matches FP32 at every depth tested.

\begin{table}[h]
\centering
\small
\begin{tabular}{llrr}
\toprule
\textbf{Config} & \textbf{Precision} & \textbf{PExact} & \textbf{GFLOPs} \\
\midrule
$H{=}3$, $n{=}2$ (peak)  & FP32 & 36.00\% & 375 \\
$H{=}1$, $n{=}4$         & INT8 & 34.25\% & 250 \\
$H{=}1$, $n{=}8$         & INT8 & 35.25\% & 500 \\
$H{=}1$, $n{=}16$        & INT8 & 36.25\% & 1{,}000 \\
$H{=}1$, $n{=}4$         & INT4 & 25.25\% & 250 \\
\bottomrule
\end{tabular}
\caption{ARC-AGI-1 depth--precision sweep (full-system, single-pass, no TTA).
INT8 at $H{=}1$,
$n_\text{sup}{=}8$ reaches 35.25\% at 500\,GFLOPs---within 0.75\,pp of the
36.00\% FP32 peak at $6\times$ fewer FLOPs.}
\label{tab:depth_arc}
\end{table}

\section{Depth × Quantization Sweep (Maze-Hard)}
\label{app:depth_maze}

Table~\ref{tab:depth_maze} shows key configurations from the Maze-Hard
depth sweep, confirming rapid saturation.

\begin{table}[ht]
\centering
\small
\begin{tabular}{llrr}
\toprule
\textbf{Config} & \textbf{Prec.} & \textbf{PExact} & \textbf{GFLOPs} \\
\midrule
$H{=}3$, $n{=}10$$^\dagger$ & FP32 & 86.80\% & 1{,}875 \\
$H{=}1$, $n{=}8$            & INT8 & 86.90\% & 500 \\
$H{=}1$, $n{=}4$            & INT8 & 84.50\% & 250 \\
$H{=}1$, $n{=}8$            & INT4 & 86.30\% & 500 \\
\bottomrule
\end{tabular}
\caption{On Maze-Hard, INT8 at $H{=}1$, $n{=}8$ matches the evaluated FP32
configuration at $3.75\times$ fewer FLOPs: depth and precision can both be
cut on this task. Depth--precision sweep; $^\dagger$evaluation configuration
($n_\text{sup}{=}10$), TRM's default test-time setting is $n_\text{sup}{=}16$.
% TODO-RERUN(E-T1): re-run at n_sup=16
}
\label{tab:depth_maze}
\end{table}

\section{Depth × Quantization Sweep (Sudoku-Extreme)}
\label{app:depth_sudoku}

Table~\ref{tab:depth_sudoku} shows key configurations from the
Sudoku-Extreme depth sweep: accuracy continues to improve with depth within
the swept range ($n_\text{sup} \le 10$).
% TODO-RERUN(E-T1): extend sweep to n_sup=16 (TRM default) to test saturation

\begin{table}[ht]
\centering
\small
\begin{tabular}{llrr}
\toprule
\textbf{Config} & \textbf{Prec.} & \textbf{PExact} & \textbf{GFLOPs} \\
\midrule
$H{=}3$, $n{=}10$$^\dagger$ & FP32 & 69.10\% & 256 \\
$H{=}4$, $n{=}10$           & FP32 & 70.30\% & 342 \\
$H{=}4$, $n{=}10$           & INT8 & 70.20\% & 342 \\
$H{=}1$, $n{=}8$            & INT8 & 55.40\% & 68 \\
$H{=}4$, $n{=}10$           & INT4 & 6.00\%  & 342 \\
\bottomrule
\end{tabular}
\caption{On Sudoku-Extreme, depth cannot be cut: INT8 at $H{=}4$, $n{=}10$
matches FP32 (70.20\% vs 70.30\%), but $H{=}1$ loses 15 points and
na\"ive INT4 loses everything at any depth. Depth--precision sweep;
$^\dagger$evaluation configuration ($n_\text{sup}{=}10$), TRM's default
test-time setting is $n_\text{sup}{=}16$.
% TODO-RERUN(E-T1): re-run at n_sup=16
}
\label{tab:depth_sudoku}
\end{table}

\section{Architecture Ablation: MLP-Mixing vs.\ Attention}
\label{app:arch_ablation}

To separate architecture from task precision we evaluate three recursive
architectures on the \emph{same} task (Sudoku-Extreme) under an identical
harness ($N{=}256$, 16 ACT steps, no TTA; Table~\ref{tab:arch_ablation}).
TRM-MLP-Mixing and TRM-Attention are the same model family at the same
full-precision accuracy ($73.8$ vs.\ $73.1$\% puzzle exact), differing only in
the token mixer; HRM~\citep{wang2025hrm} is a different recursive architecture
(separate high- and low-level modules, attention-based). Under na\"ive INT4,
TRM-MLP-Mixing collapses to $10.2$\% while both attention architectures retain
their accuracy. Since TRM-Attention matches TRM-MLP at full precision, this is
not an accuracy-headroom effect---the INT4 fragility is specific to MLP-mixing,
not the task. The carry-trajectory fidelity diagnostic grades all three
correctly ($0.35$\,/\,$0.87$\,/\,$0.98$), confirming it generalizes across
recursive architectures. HRM is also evaluated on a second task, Maze-Hard,
from the official checkpoint (\texttt{HRM-checkpoint-maze-30x30-hard},
1{,}000 test mazes, 16 ACT steps): FP32 74.3\%, INT8 74.3\%, na\"ive INT4
75.0\% and calibrated INT4 74.4\% puzzle exact, with fidelity 1.000, 0.9995,
0.993 and 0.998. Attention-HRM survives na\"ive INT4 on Maze as
TRM-Attention does, and all four fidelities clear $\tau{=}0.83$ on a
checkpoint the threshold never saw.

\begin{table}[h]
\centering
\small
\begin{tabular}{llrrr}
\toprule
\textbf{Architecture} & \textbf{Task} & \textbf{FP32} & \textbf{INT4} & \textbf{Fidelity} \\
\midrule
TRM-MLP-Mixing      & Sudoku-Extreme & 73.8 & 10.2 & 0.35 \\
TRM-Attention       & Sudoku-Extreme & 73.1 & 69.5 & 0.87 \\
HRM (diff.\ family) & Sudoku-Extreme & 47.7 & 48.4 & 0.98 \\
HRM (diff.\ family) & Maze-Hard      & 74.3 & 75.0 & 0.99 \\
\bottomrule
\end{tabular}
\caption{Only MLP-mixing collapses under na\"ive INT4; both attention
architectures survive, on the same task and, for HRM, on a second task.
Puzzle-exact (\%) and final-state carry fidelity (Sudoku rows: submission
protocol, corrected-protocol values for the two TRM variants in
Table~\ref{tab:corrected}; Maze row: official HRM checkpoint, 1{,}000
mazes). TRM-Attention matches TRM-MLP at FP32, ruling out an
accuracy-headroom confound; HRM on Sudoku sits at a lower FP32 baseline and
corroborates the pattern rather than serving as a controlled comparison.}
\label{tab:arch_ablation}
\end{table}

\section{Carry-State Diagnostic: Full Data}
\label{app:carry_traj}

We measure two carry-state quantities, computed by hooking the shared
reasoning module across all recursive calls within one inference pass.
Both are computed on real test puzzles (Maze $N{=}64$, ARC $N{=}32$,
Sudoku $N{=}256$); the ARC and Maze checkpoints are the public TRM releases,
the Sudoku TRM-MLP checkpoint is a community reproduction (see checkpoint
provenance, \S\ref{app:impl}), and all numbers below are reproduced from
those checkpoints.

\paragraph{Consecutive carry similarity (single-model).}
The mean cosine similarity between consecutive carry states
(Table~\ref{tab:carry_consec}) is task-specific but \emph{insensitive} to
compression: it is essentially identical under FP32, INT8, and INT4 on every
task (changes $\le 0.064$), and is therefore a weak failure signal. We report
it for completeness; the diagnostic below is the one we recommend.

\begin{table}[h]
\centering
\small
\begin{tabular}{lrrr}
\toprule
\textbf{Precision} & \textbf{ARC} & \textbf{Maze} & \textbf{Sudoku} \\
\midrule
FP32 & 0.415 & 0.697 & 0.806 \\
INT8 & 0.412 & 0.697 & 0.806 \\
INT4 & 0.479 & 0.699 & 0.841 \\
\bottomrule
\end{tabular}
\caption{Mean consecutive carry-state cosine similarity. The change under
INT4 is small on every task ($\le 0.064$, and $\le 0.035$ on the two tasks
where INT4 is catastrophic); the signal does not reliably
separate compression that preserves reasoning from compression that destroys
it. (Maze/Sudoku reproduced; ARC from the source run.)}
\label{tab:carry_consec}
\end{table}

\paragraph{Carry-trajectory fidelity (vs.\ full-precision reference).}
The recommended diagnostic is the cosine similarity between the quantized
model's final carry state and the FP32 model's final carry state on the same
input---how far quantization pushes the reasoning trajectory off the
full-precision path (Table~\ref{tab:carry_fidelity}). It requires only the
FP32 reference (available before deployment) and no task labels. Unlike the
consecutive signal, fidelity is \emph{graded and monotonic with severity}:
it stays $\approx$1.0 wherever INT4 is harmless (Maze, all INT8) and falls in
proportion to the accuracy damage---moderately on ARC ($0.69$, $-10$\,pp) and
catastrophically on Sudoku ($0.35$, $-64$\,pp). Per-channel calibrated INT4
\emph{recovers} fidelity in lockstep with accuracy, so the diagnostic predicts
both failure and recovery.

\begin{table}[h]
\centering
\small
\begin{tabular}{lrrr}
\toprule
\textbf{Precision} & \textbf{Maze} & \textbf{ARC} & \textbf{Sudoku} \\
\midrule
FP32              & 1.000 & 1.000 & 1.000 \\
INT8              & 1.000 & 0.999 & 0.998 \\
INT4 naïve      & 0.989 & 0.688 & 0.353 \\
INT4 calibrated   & ---   & 0.944 & 0.894 \\
\midrule
\textit{INT4 accuracy $\Delta$} & \textit{$-0.4$pp} & \textit{$-10.5$pp} & \textit{$-63.8$pp} \\
\bottomrule
\end{tabular}
\caption{Carry-trajectory fidelity (final-state cosine vs.\ FP32), submission
protocol (the accuracy deltas match Table~\ref{tab:full_results}). Monotonic
with INT4 severity (Maze $\to$ ARC $\to$ Sudoku); INT8 is never flagged;
calibrated INT4 recovers both fidelity and accuracy. Last row: INT4-naïve
puzzle-exact change vs.\ FP32.}
\label{tab:carry_fidelity}
\end{table}

\paragraph{Calibrated INT4 recovers Sudoku.}
Measured under an identical evaluation harness ($N{=}256$, 16 ACT steps, no
TTA), naïve per-tensor INT4 collapses Sudoku to $10.2$\% puzzle-exact while
per-channel calibrated INT4 recovers to $71.9$\% (vs.\ $73.8$\% FP32 under the
same harness)---i.e., the catastrophic INT4 result is specific to naïve
quantization, and calibrated INT4 is the deployable low-precision point
(Table~\ref{tab:sudoku_recover}).

\begin{table}[h]
\centering
\small
\begin{tabular}{lrrr}
\toprule
\textbf{Variant} & \textbf{PExact} & \textbf{Cell} & \textbf{Fidelity} \\
\midrule
FP32              & 73.8 & 88.9 & 1.000 \\
INT8              & 73.1 & 88.7 & 0.998 \\
INT4 naïve        & 10.2 & 67.8 & 0.353 \\
INT4 calibrated   & 71.9 & 88.2 & 0.894 \\
\bottomrule
\end{tabular}
\caption{Carry fidelity tracks accuracy across all four variants on
Sudoku-Extreme, and calibrated INT4 recovers both. Identical harness
(submission protocol, $N{=}256$, no TTA; FP32 reads $73.8$ here vs.\ $69.1$
on the full test set elsewhere, and $74.6$ under the corrected protocol of
Table~\ref{tab:corrected}).}
\label{tab:sudoku_recover}
\end{table}

\section{Structured Pruning and Knowledge Distillation}
\label{app:pruning_distill}

\paragraph{Structured pruning.}
Magnitude-based structured pruning was evaluated at 25\% and 50\% sparsity
targets across all three tasks (Table~\ref{tab:pruning}).

\begin{table*}[ht]
\centering
\small
\begin{tabular}{l rr rr rr}
\toprule
 & \multicolumn{2}{c}{\textbf{Dense (0\%)}} & \multicolumn{2}{c}{\textbf{25\% sparse}} & \multicolumn{2}{c}{\textbf{50\% sparse}} \\
\cmidrule(lr){2-3}\cmidrule(lr){4-5}\cmidrule(lr){6-7}
\textbf{Task} & \textit{PExact} & \textit{CellAcc} & \textit{PExact} & \textit{CellAcc} & \textit{PExact} & \textit{CellAcc} \\
\midrule
ARC    & 36.00\% & 87.55\% & 0.00\% & 0.27\%  & 0.00\% & 0.58\% \\
Maze   & 86.80\% & 99.52\% & 0.00\% & 86.40\% & 0.00\% & 0.00\% \\
Sudoku & 69.10\% & 87.47\% & 0.00\% & 50.01\% & 0.00\% & 37.81\% \\
\bottomrule
\end{tabular}
\caption{Structured pruning results. Even 25\% sparsity destroys puzzle-level
reasoning across all tasks. Cell accuracy partially survives on Maze (86.40\%)
and Sudoku (50.01\%), indicating that token prediction survives while global
constraint satisfaction does not.}
\label{tab:pruning}
\end{table*}

\paragraph{Knowledge distillation.}
Student models (hidden=256, 1 layer, 1-cycle) were trained via KL-divergence
distillation from the full teacher (Table~\ref{tab:distill}).

\begin{table}[ht]
\centering
\small
\begin{tabular}{lrr rr}
\toprule
\textbf{Task} & \textbf{Teacher} & \textbf{Student} & \textbf{PExact} & \textbf{CellAcc} \\
\midrule
Maze   & 6.82M & 855K & 0.00\% & 87.25\% \\
Sudoku & 5.03M & 745K & 0.00\% & 54.77\% \\
\bottomrule
\end{tabular}
\caption{Knowledge distillation results. Student models (12--15\% of teacher
params) learn token-level patterns but fail entirely at puzzle-level
reasoning, suggesting the recursive structure is functionally necessary.}
\label{tab:distill}
\end{table}

\section{Linear-Attention Approximation (Maze)}
\label{app:linattn}

Replacing softmax attention with ELU feature-map linear attention
($\mathcal{O}(n)$ vs.\ $\mathcal{O}(n^2)$) on Maze illustrates the same
cell-vs-puzzle split as quantization: the swap preserves token-level accuracy
but destroys puzzle-level reasoning. Evaluated at $H{=}3$, $n_\text{sup}{=}1$
(hence the 78.50\% baseline rather than the full-depth 86.80\%): zero-shot,
cell accuracy holds at 87.3\% while puzzle-exact falls to 0.00\% (from
78.50\% / 99.40\%); brief retraining
(200 steps) recovers cell accuracy (87.5\%) but not puzzle-exact (0.00\%).
This is a third intervention---alongside pruning and
distillation---under which local prediction survives while global constraint
satisfaction collapses. Sudoku-Extreme (MLP-mixing) has no attention layers
and is not applicable.

\section{QAT Configurations}
\label{app:qat}

Table~\ref{tab:qat} reports the six quantization-aware-training configurations
of \S\ref{sec:qat}: two objectives at three learning rates each, 1{,}000 steps
at batch 32 from the calibrated-INT4 initialization (72.3\% at step 0).

\begin{table}[H]
\centering
\small
\begin{tabular}{@{}lrrr@{}}
\toprule
\textbf{Final pass@1 (1{,}000 steps)} & lr $10^{-5}$ & lr $10^{-4}$ & lr $10^{-3}$ \\
\midrule
Cross-entropy      & 53.9\% & 32.4\% & 2.3\% \\
Distillation (KD)  & 53.9\% & 37.1\% & 7.8\% \\
\bottomrule
\end{tabular}
\caption{QAT from the calibrated-INT4 initialization (72.3\% at step 0). All
six configurations degrade the model they start from.}
\label{tab:qat}
\end{table}

\section{Energy per Inference}
\label{app:energy}

Estimated energy follows the FLOPs counts under a Cortex-M55 power model
($\sim$1\,mJ/GFLOP): ARC-AGI-1 at full depth ($\sim$3{,}000\,GFLOPs/puzzle)
draws $\sim$3{,}000\,mJ/puzzle, versus $\sim$500\,mJ at the reduced
configuration ($H{=}1$, $n_\text{sup}{=}8$). Sudoku-Extreme
($\sim$256\,GFLOPs at default depth) draws $\sim$256\,mJ/puzzle. These are
analytical estimates under the same FLOPs-based model. The model is
precision-blind---it assigns no separate energy-per-operation term to FP32
vs.\ INT8---so the $6\times$ energy saving follows entirely from the
$6\times$ FLOPs (cycle) reduction, not from quantization.

\section{Context-Length Truncation}
\label{app:context}

Because attention cost scales as $\mathcal{O}(T^2)$, we tested zero-padding the
input beyond a truncated context. Truncation is destructive on every task
(Table~\ref{tab:context}): halving the sequence length takes Maze and Sudoku to
zero and costs ARC nearly ten points. There is no cheap context shortcut---the
full window is load-bearing.

\begin{table}[H]
\centering
\small
\begin{tabular}{lrrr}
\toprule
\textbf{Context} & \textbf{ARC} & \textbf{Maze} & \textbf{Sudoku} \\
\midrule
full (900 / 81) & 36.00 & 78.50 & 28.40 \\
$\sim$50\%      & 26.50 & 0.00  & 0.00  \\
$\sim$25\%      & 10.75 & ---   & ---   \\
\bottomrule
\end{tabular}
\caption{The input cannot be truncated: Maze and Sudoku collapse to 0 at
50\% context and ARC degrades severely, so the sequence length in the
memory budget is not a free parameter. Puzzle-exact accuracy under input
context truncation, evaluated at $H{=}3$, $n_\text{sup}{=}1$ (the
full-context rows match the $n{=}1$ column of
Tables~\ref{tab:maze_sweep_detail}--\ref{tab:sudoku_sweep_detail}, which is
why they sit below the full-depth baselines quoted elsewhere).}
\label{tab:context}
\end{table}

\section{Implementation Details}
\label{app:impl}

\paragraph{Checkpoint provenance.}
The Sudoku TRM-MLP checkpoint is the alphaXiv community reproduction of TRM,
whose model card reports 79.37\% puzzle exact vs.\ 87.4\% in the original
paper. Our Sudoku claims are therefore relative comparisons between
compression variants evaluated at matched checkpoints, not absolute-accuracy
claims against the original release.
% CAMERA-READY(E-T5): from-scratch retrain

\paragraph{Quantization.}
INT8 and INT4 PTQ were applied using \texttt{bitsandbytes}
v0.41~\citep{dettmers2022llmint8} with \texttt{load\_in\_8bit=True} and
\texttt{load\_in\_4bit=True} respectively. Per-channel calibration for
INT4 calibrated used 128 calibration puzzles drawn from the training set.

\paragraph{Carry-state extraction.}
$s_h$ was computed by registering a forward hook on the carry-state update
function $g_\phi$ to capture $Z_h$ at each outer cycle. Cosine similarity
was computed token-wise and averaged across the sequence dimension and
across all puzzles in the evaluation set.

\paragraph{QAT.}
The headline QAT runs (\S\ref{sec:qat}) initialize from the calibrated-INT4
checkpoint and fine-tune for 1{,}000 steps at batch 32, under cross-entropy
and token-distillation objectives at learning rates $10^{-5}$, $10^{-4}$, and
$10^{-3}$, with the deep-supervision ACT loop. A shorter probe (100
steps, $\text{lr}{=}10^{-5}$, cross-entropy, batch 4, from the na\"ive INT4
checkpoint) is the held-out run cited in \S\ref{sec:qat}. Training and
evaluation used the Modal cloud platform.

\paragraph{ONNX export and edge deployment.}
Models were exported to ONNX format using \texttt{torch.onnx.export} for
deployment via ONNX Runtime and Qualcomm AI Hub. The ONNX export produces
a single-step model (\texttt{TRMBackboneStep}) that executes one
H-cycle step, with the outer recursion loop managed by the inference
harness.
